# Supplementary material for: Triple point fermions in ferroelectric GeTe
Source: arXiv:2012.02010 source file (2020-12-03)
Supplement: Supplementary file 1 [file Supplementary.pdf]

# SUPPLEMENTARY INFORMATION
# "Triple point fermions in ferroelectric GeTe"


Juraj Krempaský[1], Laurent Nicolaï[2], Martin Gmitra[3], Houke Chen[4], Mauro Fanciulli[5], Eduardo B. Guedes[1], Marco Caputo[1], Milan Radović[1], V. V. Volobuev[6,7], Ondřej Caha[8], Gunther Springholz[9], Jan Minár[2], J. Hugo Dil[1,10]

[1]*Photon Science Division, Paul Scherrer Institut, CH-5232 Villigen, Switzerland*

[3]*New Technologies-Research Center University of West Bohemia, Plzeň, Czech Republic*

[3]*Institute of Physics, P. J. Šafárik University in Košice, Park Angelinum 9, 040 01 Košice, Slovakia*

[4]*Department of Physics, Tsinghua University, Beijing 100084, China*

[5]*LPMS, Université de Cergy-Pontoise, 95031 Cergy-Pontoise, France*

[6]*International Research Centre MagTop, Institute of Physics, Polish Academy of Sciences, Aleja Lotnikow 32/46, PL-02668 Warsaw, Poland*

[7]*National Technical University "KhPI", Kyrpychova Str. 2, 61002 Kharkiv, Ukraine*

[8]*Department of Condensed Matter Physics, Masaryk University, Kotlářská 267/2, 61137 Brno, Czech Republic*

[9]*Institut für Halbleiter-und Festkörperphysik, Johannes Kepler Universität, A-4040 Linz, Austria*

[10]*Institut de Physique, École Polytechnique Fédérale de Lausanne, CH-1015 Lausanne, Switzerland*


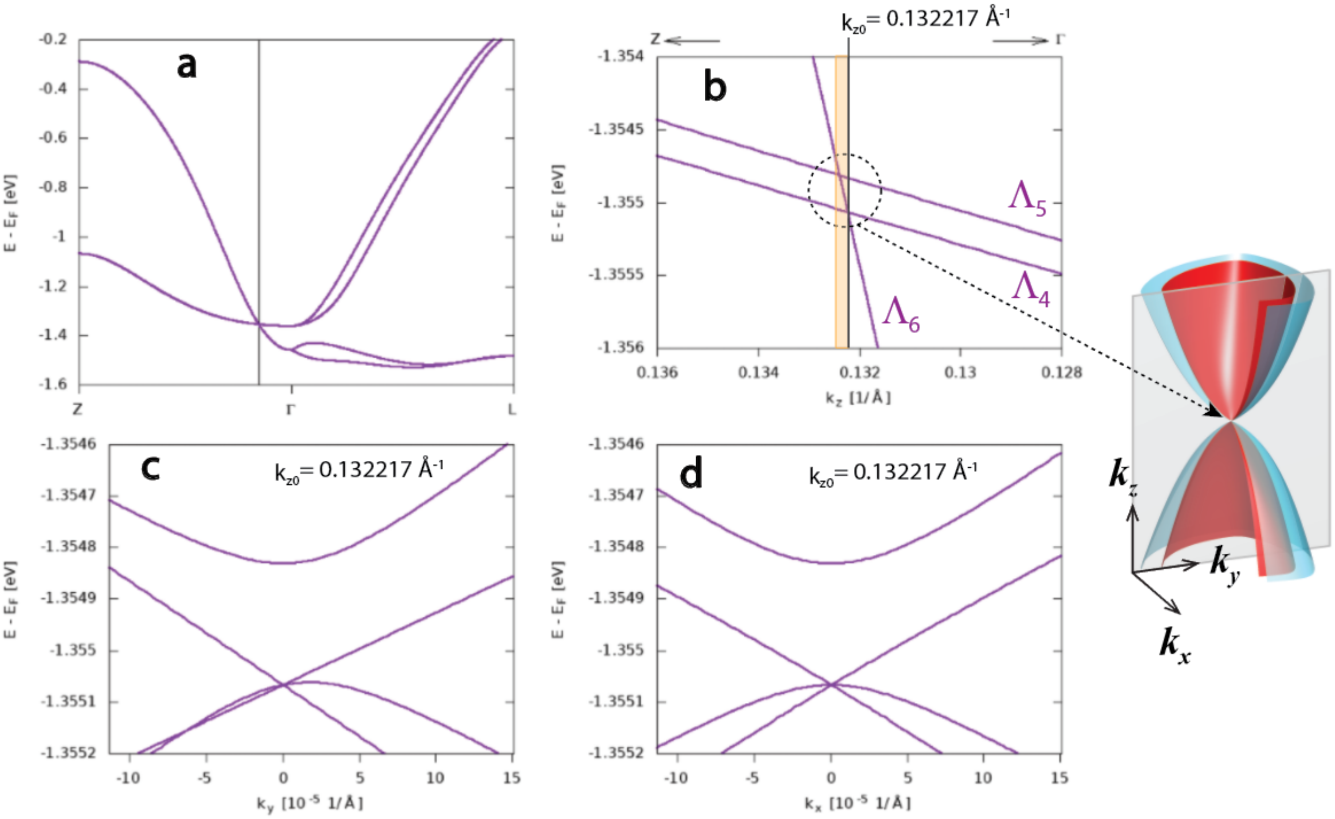


FIG. S1. (a) $\alpha$-GeTe(111) calculated band structure along the Γ-Z and Γ-L directions. (b) Formation of a TP pair by spin-degenerate band $\Lambda_6$ and two spin split bands $\Lambda_{4,5}$ (also seen in Fig. 2b in main text). (c,d) Close-up of band structure around the TP along $k_y$ ($\overline{M\Gamma M}$) and $k_x$ ($\overline{K\Gamma K}$) directions as denoted inside the 3D TP cartoon on the right. A movie visualising the $k_z$-dependency of (c) and (d) within the region indicated by an orange box in (b) is available in animated gif format online.

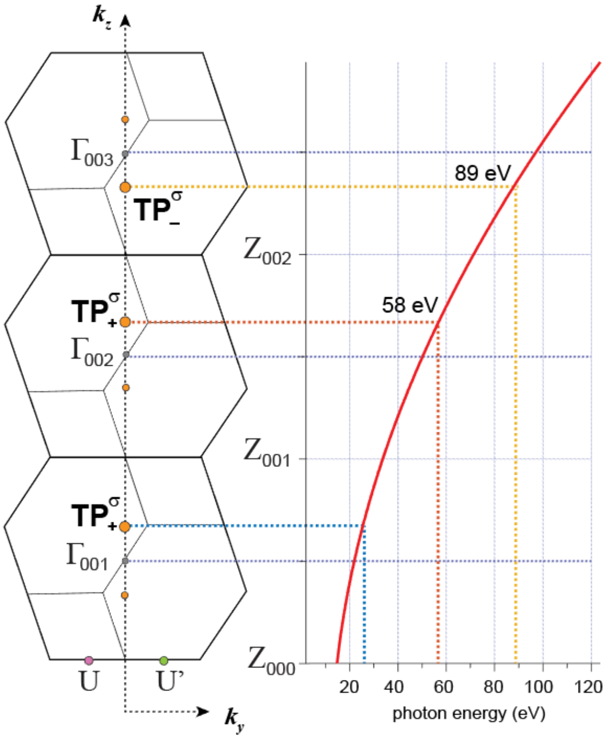


FIG. S2. Schematic diagram for $k_z$ mapping along the ZΓZ direction showing the $\mathrm{TP}^\sigma_+$ around 30 and 58 eV; and $\mathrm{TP}^\sigma_-$ around 89 eV photon energy. The normalized $k_z$ values are based on an inner potential $V_0 = -8.0$ eV and $\alpha$-GeTe(111) surface-relaxed lattice constant of 4 Å based on x-ray photoelectron diffraction measurements (to be published and courtesy of M. Muntwiler, Pearl beamline, Swiss Light Source).

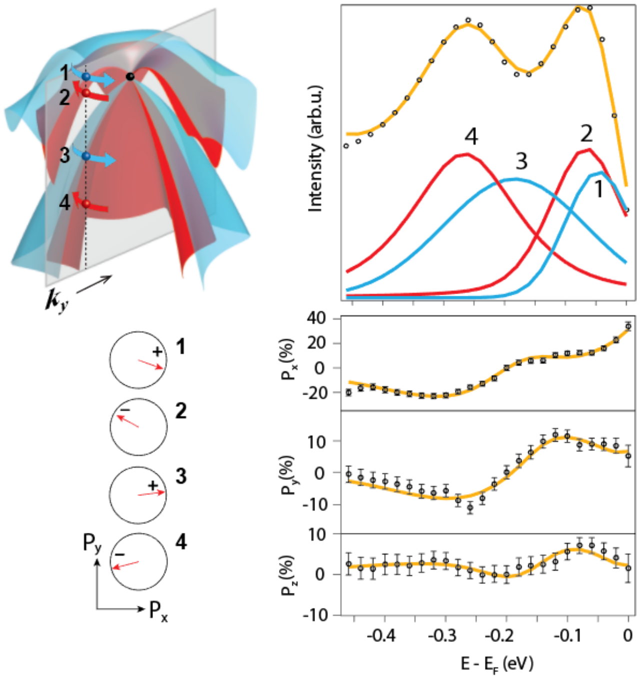


FIG. S3. (a) SARPES EDC total intensity and related $P_{x,y,z}$ spin polarizations measured at the Z-point (22 eV) with the same experimental geometry as for the triple-point in Fig.4 of main text. The Rashba-type spin texture with corresponding $\mathrm{B}_{1,2,3,4}$ bulk band fitting is indicated in red-blue. The 3D cartoon shows the EDC cut and corresponding spin vectors 1-4 with characteristic Rashba-type (+-+-) $P_x$ spin texture.

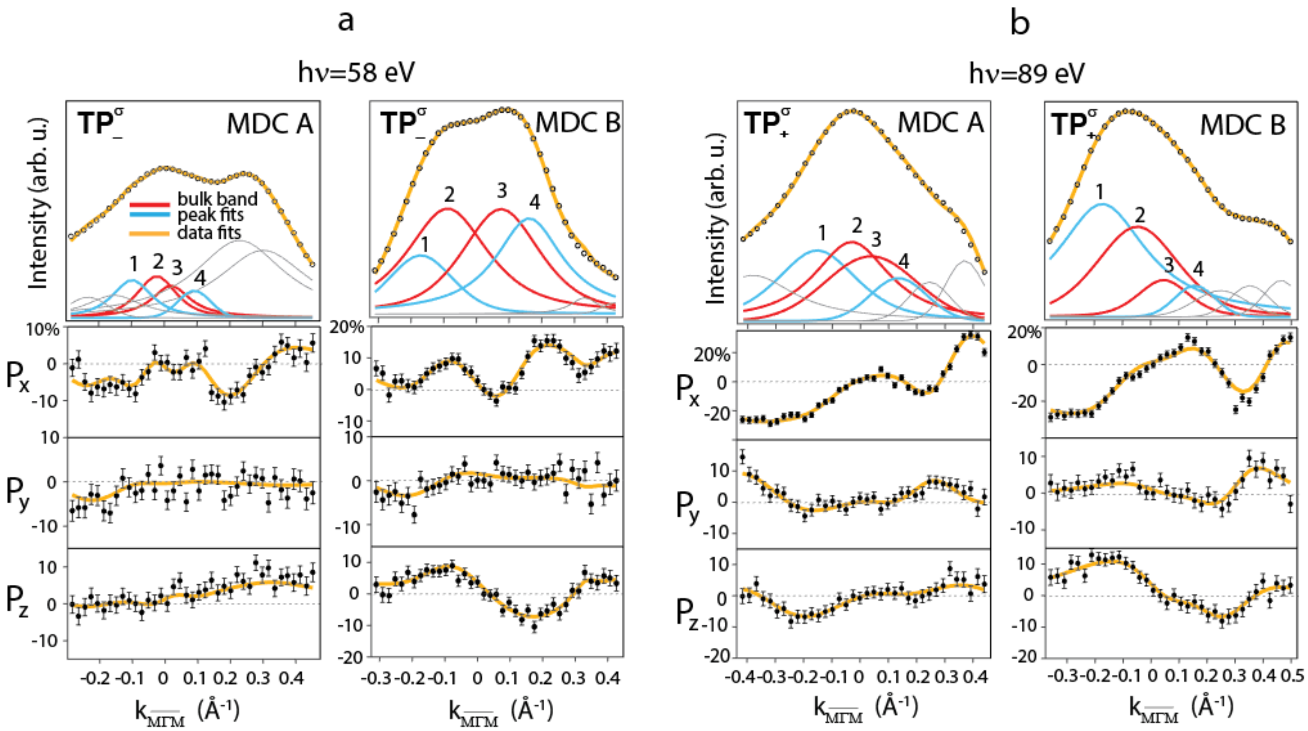


FIG. S4. (a) SARPES intensities and 3D spin polarization fitting for $TP^{\sigma}_{+}$ (h$\nu$=58 eV) along the U-A-U' direction, to be compared with SARPES data along U'-A-U in Fig. 5b of the main text (sample rotated 180°). (b) The same for $TP^{\sigma}_{-}$ measured at h$\nu$=89 eV. Red and blue curves indicate the $B_{1,2,3,4}$ peak fitting.
